# Supplementary material for: Logistic-Normal Likelihoods for Heteroscedastic Label Noise
Source: arXiv:2304.02849 source file (2023-08-14)
Supplement: Supplementary file 1 [file histograms_of_mse.tex]

\begin{figure}
    \centering
    \includegraphics[width=.49\textwidth]{Figures/supplementary/hist_mse-50-bins.pdf}
    \caption{No Caption yet}
    \label{fig:my_label}
\end{figure}
